# Supplementary material for: 3D-SceneDreamer: Text-Driven 3D-Consistent Scene Generation
Source: arXiv:2403.09439 source file (2024-03-14)
Supplement: Supplementary file 1 [file X_suppl.tex]

\clearpage
\setcounter{page}{1}
\maketitlesupplementary

\appendix

\setcounter{equation}{0}

\section{Latent Diffusion Model Revisted}
Diffusion models (DM)~\cite{kawar2022denoising} is a type of probabilistic model designed to estimate the underlying data distribution $p(x)$ by learning to denoise a noised input data $x_t$ that is constructed by adding a scaled gaussian noise into the input data $x$. 
%TEME: the iteratively removing noise from standard normal gaussian is the sampling not the learning process 

% This process can be thought of as the inverse of learning a fixed Markov chain with a length of $T$.
Given input sample $\boldsymbol{x} \sim p(\boldsymbol{x})$, the noised data is obtained as $\boldsymbol{x}_t = \alpha_t \boldsymbol{x} + \sigma_t \boldsymbol{\epsilon}, \boldsymbol{\epsilon} \sim \mathcal{N}(0, \mathbf{I})$, DMs are trained using a simplified objective function that learns to predict the noise $\boldsymbol{\epsilon}$ that constructs $\boldsymbol{x}_t$ from $\boldsymbol{x}$ using a denoising auto-encoder network $\boldsymbol{\epsilon}_{\theta}$: 

% can then be viewed as predicting the denoised variant of the input $\boldsymbol{x}_t$ by training a sequence of equal-weighted denoising auto-encoders $\epsilon_\theta$.
% The training objective can be simplified to:
\begin{equation}
    \mathcal{L}_{D M}=\mathbb{E}_{\boldsymbol{x} \sim p(x), \boldsymbol{\epsilon} \sim \mathcal{N}(0,1), t}\left[\left\|\boldsymbol{\epsilon}-\boldsymbol{\epsilon}_\theta\left(\boldsymbol{x}_t, t\right)\right\|_2^2\right]
\end{equation}
% where $\boldsymbol{c}$ is the optical conditioning information, such as a text prompt or a visual guidance (\eg depth image, and mask image).
\par
Latent diffusion models(LDM)~\cite{stablediffusion} apply the diffusion process in compressed latent space, unlike pixel-space diffusion models that operate directly on pixel space. With this, it not only lowers the computational and memory cost that enables high-resolution image generation but also allows the generation of high-fidelity images. 
LDMs first train a variational autoencoder (VAE) with encoder $\mathcal{E}$ and decoder $\mathcal{D}$, that transforms the input image $\boldsymbol{x}$ into a low-dimensional latent embedding $\boldsymbol{z}$.
Then, it combines the input conditions $\boldsymbol{s}$ to train a diffusion model in the latent space.
The LDM training objective is given as:
\begin{equation}
    \mathcal{L}_{L D M}=\mathbb{E}_{\mathcal{E}(\boldsymbol{x}), \boldsymbol{\epsilon} \sim \mathcal{N}(0,1), t}\left[\left\|\boldsymbol{\epsilon}-\boldsymbol{\epsilon}_\theta\left(\boldsymbol{z}_t, \tau(\boldsymbol{s}), t\right)\right\|_2^2\right]
\end{equation}
where $\tau$ indicates the conditional encoder.

\section{Network Details}
\subsection{Scene Representation}
\noindent{\textbf{Image Encoder.}} We use the pre-trained DINO-ViT-B/16 as our image encoder. 
This model is transformer-based, which has $12$ layers and the hidden dimension of the transformer is $768$. 
For our model, the input image resolution is $512$, thus it leads to $1024$ spatial tokens in the vision transformer. 
The original DINO is trained with a resolution of $224 \times 224$, thus the positional embedding has a size of 196.
We thus use bilinear extrapolation to extrapolate it to the desired size.

\par
\noindent{\textbf{3D Feature Volume.}} We back project the image feature map along every ray to get 3D feature volume $\boldsymbol{V}$ with dimensions $S \times S \times S \times D$ where $S$ is the resolution of feature grid and we use $S = 64$ and $D = 256$. 
This is because we have found that $K = 64$ provides reasonable performance while avoiding out-of-memory problems.
\par

\noindent{\textbf{Feature Aggregation.}}
After getting the 3D feature volume, we get the tri-plane features through three separate networks.
Taking $xy$-plane as an example, we will describe how to obtain $\mathbf{M}_{xy}$ from feature volume $\mathbf{V}$.
Specifically, we perform an average pooling operation on the z-axis to get the $\mathbf{A}_{xy} \in \mathbb{R}^{S \times D}$.
After that, we transform $\mathbf{A}_{xy}$ into the weight vector $w_{xy} \in \mathbb{R}^{S \times 1}$ via an MLP and softmax operator.
Finally, we can do a weighted summation of the 3D feature volume on the z-axis to get $\mathbf{M}_{xy}$.
The features of the other two planes can be derived by calculating them in a similar way.

\par
\noindent{\textbf{Implicit Radiance Field Decoder.}}
The implicit radiance field decoder consists of an 8-layer fully connected MLP with a hidden dimension of 128 and LeakyReLU activations. The input position $\boldsymbol{x}$ and viewing direction $\boldsymbol{d}$ are positionally encoded. The position $\boldsymbol{x}$ is connected to the tri-plane feature $\mathbf{M}_p$ as input to the first layer. The conditioning features are provided as skip connections to the third layer, and the observation dimension features are pooled to the fourth layer. Two additional MLP layers with a hidden dimension of 128 output 3-channel color values $\boldsymbol{c}$ for each sample point, based on the position-encoded viewing direction and the output feature of the fourth MLP layer.

% The implicit radiance field decoder consists of $7$ fully connected layers with a hidden dimension of 128 and LeakyReLU activations.
% We positionally encode the input position $\boldsymbol{x}$ and the viewing direction $\boldsymbol{d}$.
% Then, we connect the position $\boldsymbol{x}$ with the tri-plane feature $\mathbf{M}_p$ as input to the first layer of the MLP.
% We also provide the conditioning features as skip connections to the third layer of the MLP, the features along the observation dimension are pooled to the fourth layer of the MLP.
% We further use two additional MLP layers with a hidden dimension of 128 to output 3-channel color values $\boldsymbol{c}$ for each sample point, conditional on the position-encoded viewing direction and the output feature of the fourth MLP layer.

\subsection{Generative Refinement}
\noindent{\textbf{Feature Adapter.}} Our proposed feature adapter is lightweight and straightforward, consisting of four feature extraction blocks and three downsampling blocks for changing the feature resolution. 
The original condition input has a resolution of $512 \times 512$. We employ the pixel unshuffle operation to downsample it to $64 \times 64$. In each scale, one convolution layer and two residual blocks are used to extract the condition feature.
Finally, we obtain multi-scale condition features.
The condition feature is then added to the encoded feature at each scale.

\section{Implementation Details}
\label{sec:addition_implement}

\subsection{Differentiable Depth Image-Based Rendering}
To generate novel views, we propose to use differentiable depth image-based rendering (DIBR)~\cite{jaderberg2015spatial} to construct a supporting database $\mathcal{S}=\{[\mathbf{I}_i, \mathbf{D}_i, \mathbf{T}_i]\}_{i=1}^N$ within the neighborhood of the initial camera pose.
Specifically, for each pixel $p$ in image $\mathbf{I}_0$, and their depths, we can compute their corresponding pixels $p_{0 \rightarrow i}$ in the novel view $i$ as well as the depth values $d_{0\rightarrow i}$:

\begin{equation}
    [p_{0\rightarrow i},d_{0\rightarrow i}]^\top  \sim \mathbf{KT} _{i}\mathbf{T} _0^{-1}\mathbf{K} ^{-1}[p,\mathbf{D} _0(p)]^\top  
\end{equation}

\noindent where $\mathbf{K}$ denotes the manually set camera intrinsic matrix, and $\mathbf{T}_i$ indicates indicate the camera pose in view $i$.
To conveniently describe the surrounding poses, we use spherical coordinates $(\theta, \phi, r)$ to obtain the poses in the sample subset $\mathcal{S}$.
To facilitate the calculation of $\mathbf{T}_i$, we assume that the surrounding cameras are located on a sphere centered on the center of the initial camera.
We then describe them using spherical coordinates $(\theta_i, \phi_i, r_i)$,  where $\theta_i$,  $\phi_i$, and $r_i$ denote the polar angle, azimuth angle, and radius of view $i$, respectively.
With these support $N$ views, along with the initial view $\mathbf{I}_0$, we can then train a tri-planar NeRF as the initialized 3D scene representation.

\subsection{Scene Representation}
\noindent{\textbf{Unbounded Scene Handling.}} To deal with unbounded scenes, we adopt a scene parameterization similar to the contraction of Mip-NeRF360~\cite{barron2022mip}, which maps each point to $[-2,2]$ space before querying:

\begin{equation}
\mathcal{F}_{con}(\mathbf{x})= \begin{cases}\mathbf{x} & \text { if }\|\mathbf{x}\|_{\infty} \leq 1 \\ \left(2-\frac{1}{\|\mathbf{x}\|_{\infty}}\right)\left(\frac{\mathbf{x}}{\|\mathbf{x}\|_{\infty}}\right) & \text { otherwise. }\end{cases}
\end{equation}

Here we use the $L_{\infty}$ norm to fully utilize the square bounding boxes of our scene representation. 
To address the issue of fixed capacity models being unable to represent long trajectories, we dynamically create new representations when the camera moves beyond the current space. 
Each new representation is centered at the previous last camera position. 
We supervise these representations using a subset of generated frames, including the current representation's frames and the previous $N$ frames for overlap. This ensures a consistent reconstruction of the radiance field. Additionally, we blend the rendered colors together to enhance multiview consistency.

\subsection{Training Details}
We use an AdamW optimizer with an initial learning rate of $5e^{-4}$ and a learning rate warm-up strategy to increase the learning rate to the value of $5e^{-4}$ and then decrease it to a final learning rate of $5e^{-6}$.
We also apply a gradient clip of 1 to ensure the stability of the training process.
we refine the unified 3D representation for 800 iterations per add frame. The whole optimization takes 3 to 4 hours for 200 frames on 4 A100 GPUs.
Note that we alternated between fine-tuning the refinement model and the unified representation whenever new keyframes were added, and then optimized the unified representation after the new data was added to the supporting database.

\begin{table}[t!]
\centering
\resizebox{\columnwidth}{!}{%
\begin{tabular}{c|cccc}
\toprule
Pose Num &
  \cellcolor[HTML]{FEF1F1}\textbf{DE} &
  \cellcolor[HTML]{FEF1F1}\textbf{CE} &
  \cellcolor[HTML]{F0FBEF}\textbf{SfM rate} &
  \cellcolor[HTML]{F0FBEF}\textbf{CLIP Score} \\ \midrule
N=0  & 0.49          & 0.891          & 0.41          & 23.12          \\
N=2  & 0.28          & 0.632          & 0.49          & 25.18          \\
N=4  & 0.23          & 0.485          & 0.56          & 25.97          \\
N=8  & \textbf{0.14} & \textbf{0.179} & \textbf{0.86} & \textbf{28.71} \\
N=12 & 0.19          & 0.253          & 0.61          & 29.12          \\ \bottomrule
\end{tabular}%
}
\vspace{-3mm}
\caption{Ablation on the initial number of viewpoints.}
\vspace{-2mm}
\label{tab:ablation_pose_num}
\end{table}
\begin{table}[t!]
\centering
\resizebox{\columnwidth}{!}{%
\begin{tabular}{l|cccc}
\toprule
\textbf{Inputs} &
  \cellcolor[HTML]{FEF1F1}\textbf{DE} &
  \cellcolor[HTML]{FEF1F1}\textbf{CE} &
  \cellcolor[HTML]{F0FBEF}\textbf{SfM rate} &
  \cellcolor[HTML]{F0FBEF}\textbf{CS} \\ \midrule
Course Image     & 0.71          & 1.618          & 0.61          & 23.41          \\
+depth map       & 0.68          & 0.646          & 0.42          & 28.18          \\
+depth feature   & 0.49          & 0.495          & 0.50          & 23.97          \\
+feature adapter & \textbf{0.19} & \textbf{0.198} & \textbf{0.86} & \textbf{28.71} \\ \bottomrule
\end{tabular}%
}
\vspace{-3mm}
\caption{Ablation on the conditional input of the refine model.}
\vspace{-2mm}
\label{tab:ablation_feature}
\end{table}
\begin{table}[t!]
\centering
\resizebox{\columnwidth}{!}{%
\begin{tabular}{l|cccc}
\toprule
\textbf{Method} &
  \cellcolor[HTML]{F0FBEF}\textbf{CS$\uparrow$} &
  \cellcolor[HTML]{FEF1F1}\textbf{BRISQUE$\downarrow$} &
  \cellcolor[HTML]{FEF1F1}\textbf{NIQE$\downarrow$} &
  \cellcolor[HTML]{F0FBEF}\textbf{IS$\uparrow$} \\ \midrule
CLIP-Mesh~\cite{CLIP_Mesh}       & 27.16          & 49.26          & 6.15          & 1.09          \\
DreamFusion~\cite{dreamfusion}     & 23.15          & 31.54          & 9.47          & 1.12          \\
ProlificDreamer~\cite{Prolificdreamer} & 21.58          & 62.02          & 8.02          & 1.20          \\
\rowcolor[HTML]{EFEFEF} 
Ours            & \textbf{28.12} & \textbf{24.15} & \textbf{4.96} & \textbf{2.62} \\ \bottomrule
\end{tabular}
}
\vspace{-3mm}
\caption{\textbf{Comparision with text-to-object methods.} We compare our method with recent text-driven 3D generation methods~\cite{dreamfusion, Prolificdreamer, CLIP_Mesh}. Metrics on visual quality are illustrated.}
\label{tab:compare_to_object}
\vspace{-2mm}
\end{table}
\begin{figure*}[t]
    \centering
    \includegraphics[width=1.0\textwidth]{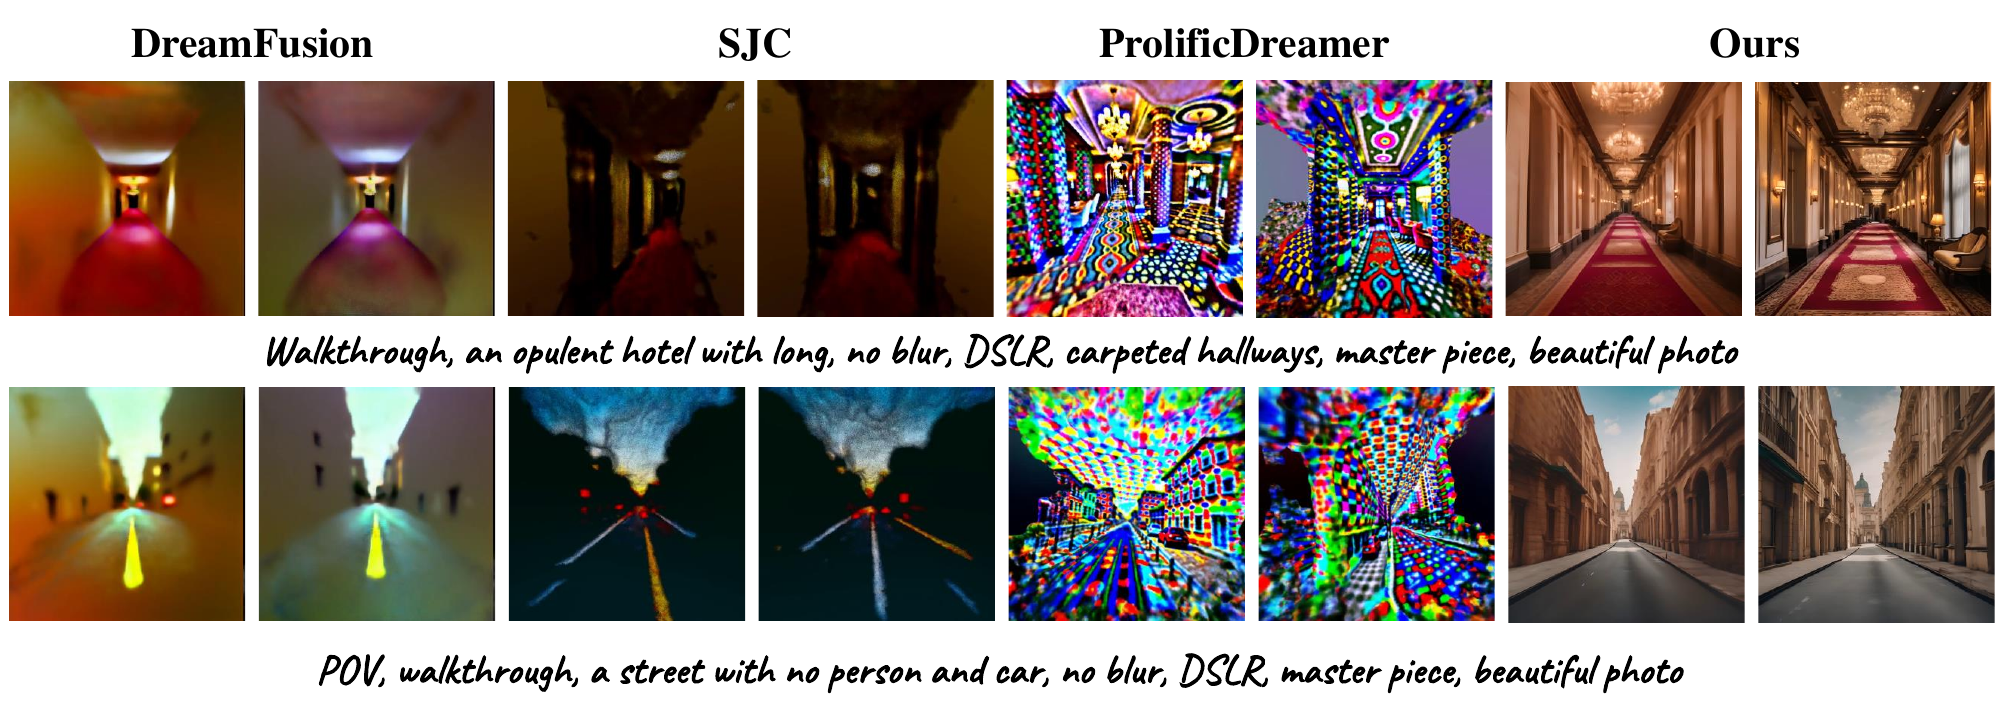}
    \vspace{-3mm}
    \caption{Compare to previous text-to-3D object methods~\cite{SJC, Prolificdreamer, dreamfusion}.}
    \vspace{-2mm}
    \label{fig:text-to-object-supp}
\end{figure*}
\begin{figure}[t]
    \centering
    \includegraphics[width=0.48\textwidth]{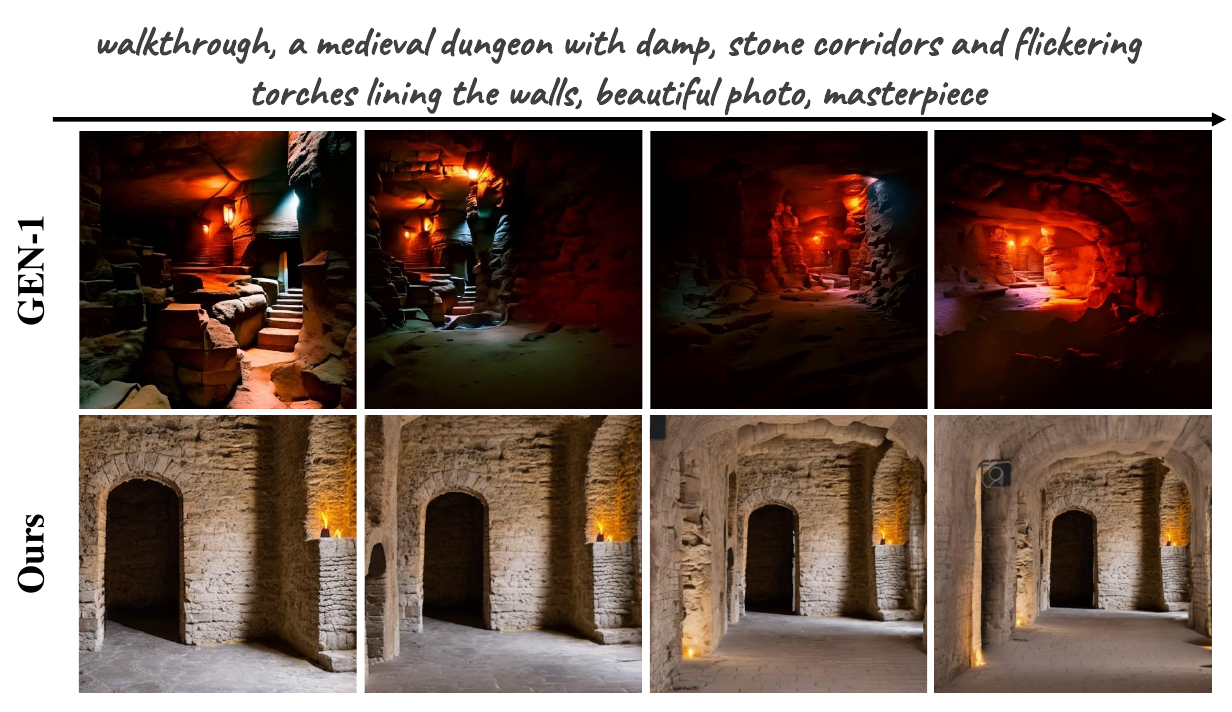}
    \vspace{-2mm}
    \caption{Comparision with video-to-video transition method GEN-1.}
    \vspace{-2mm}
    \label{fig:GEN-1}
\end{figure}
\begin{figure}[t]
    \centering
    \includegraphics[width=0.48\textwidth]{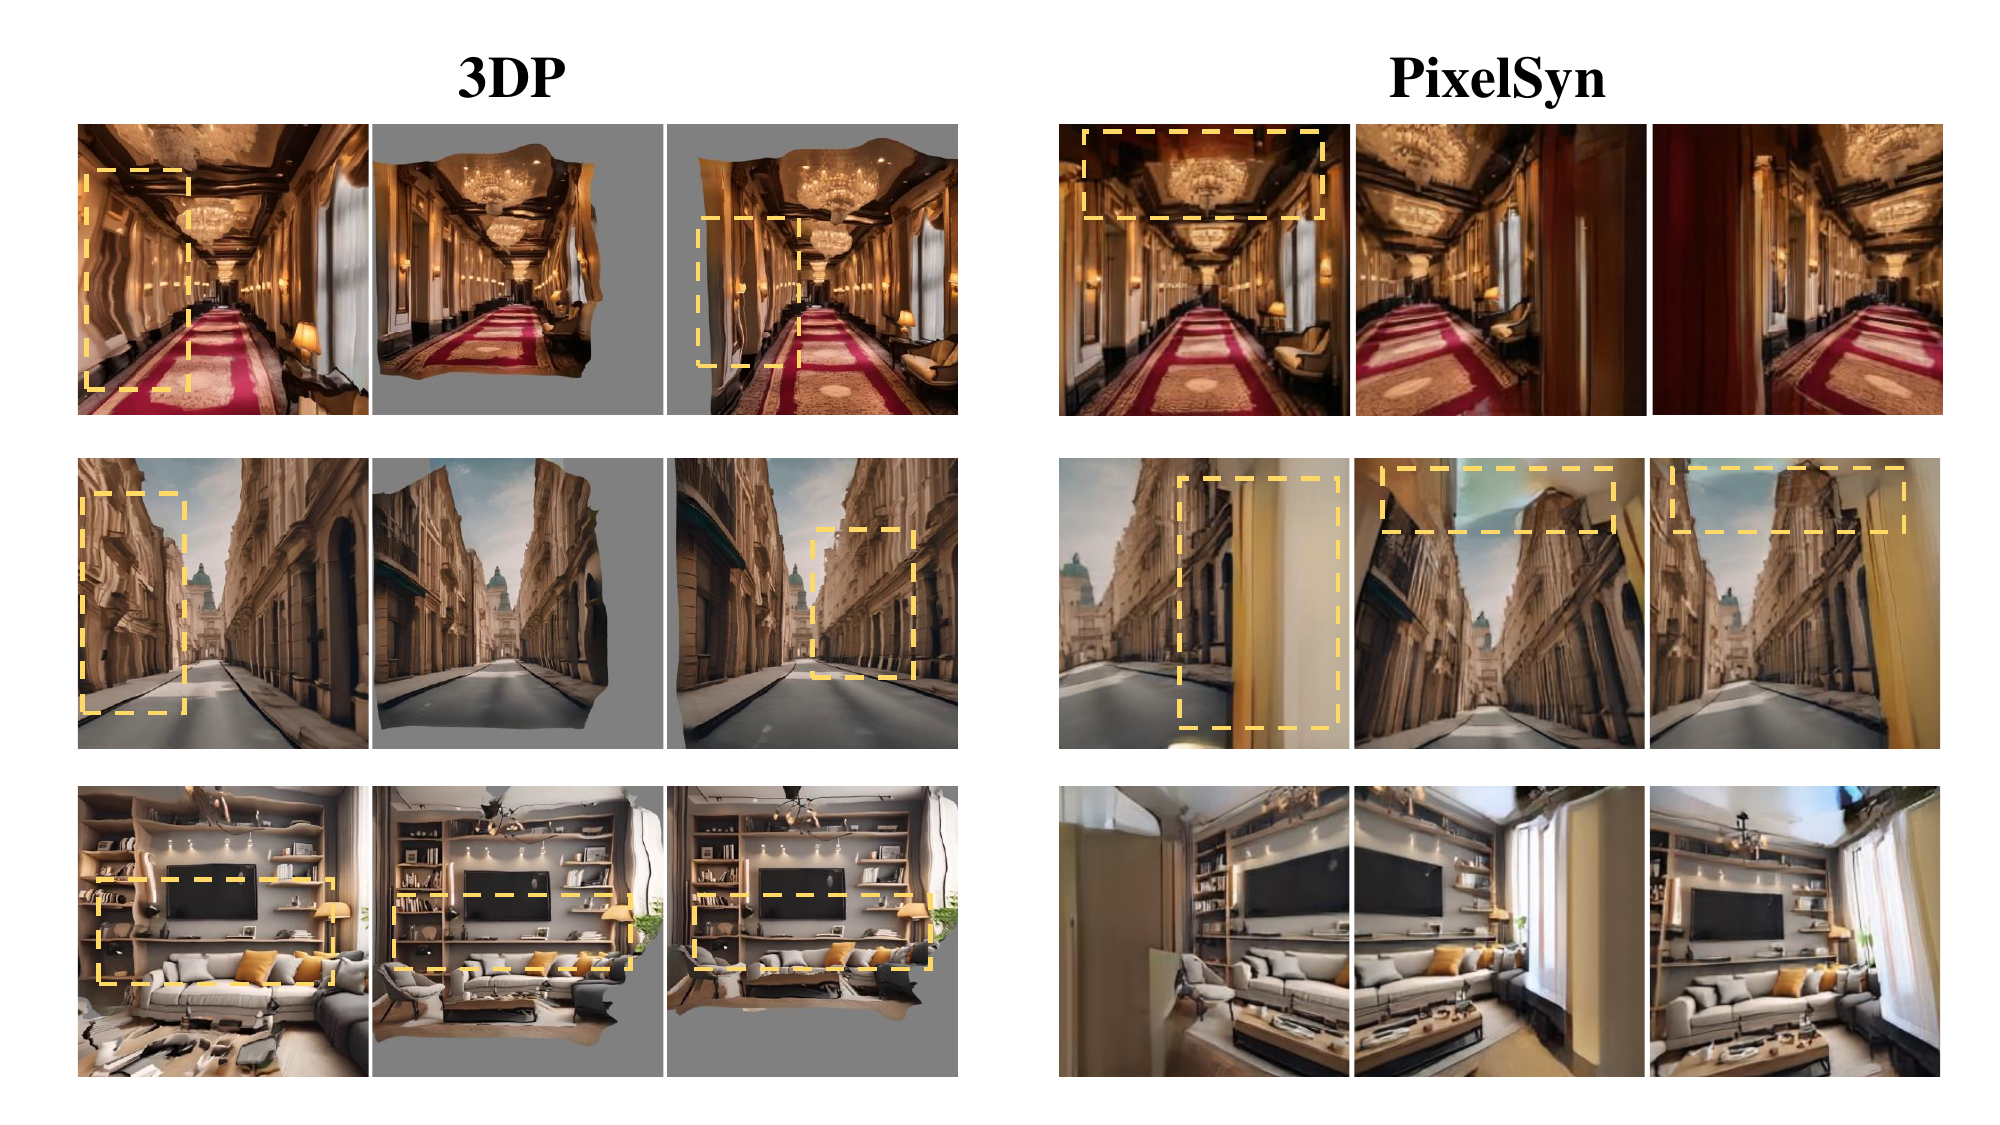}
    \vspace{-3mm}
    \caption{Visualization results of the image-guided scene generation approaches.}
    \vspace{-2mm}
    \label{fig:3dp_supp}
\end{figure}
\begin{figure*}[t]
    \centering
    \includegraphics[width=1.0\textwidth]{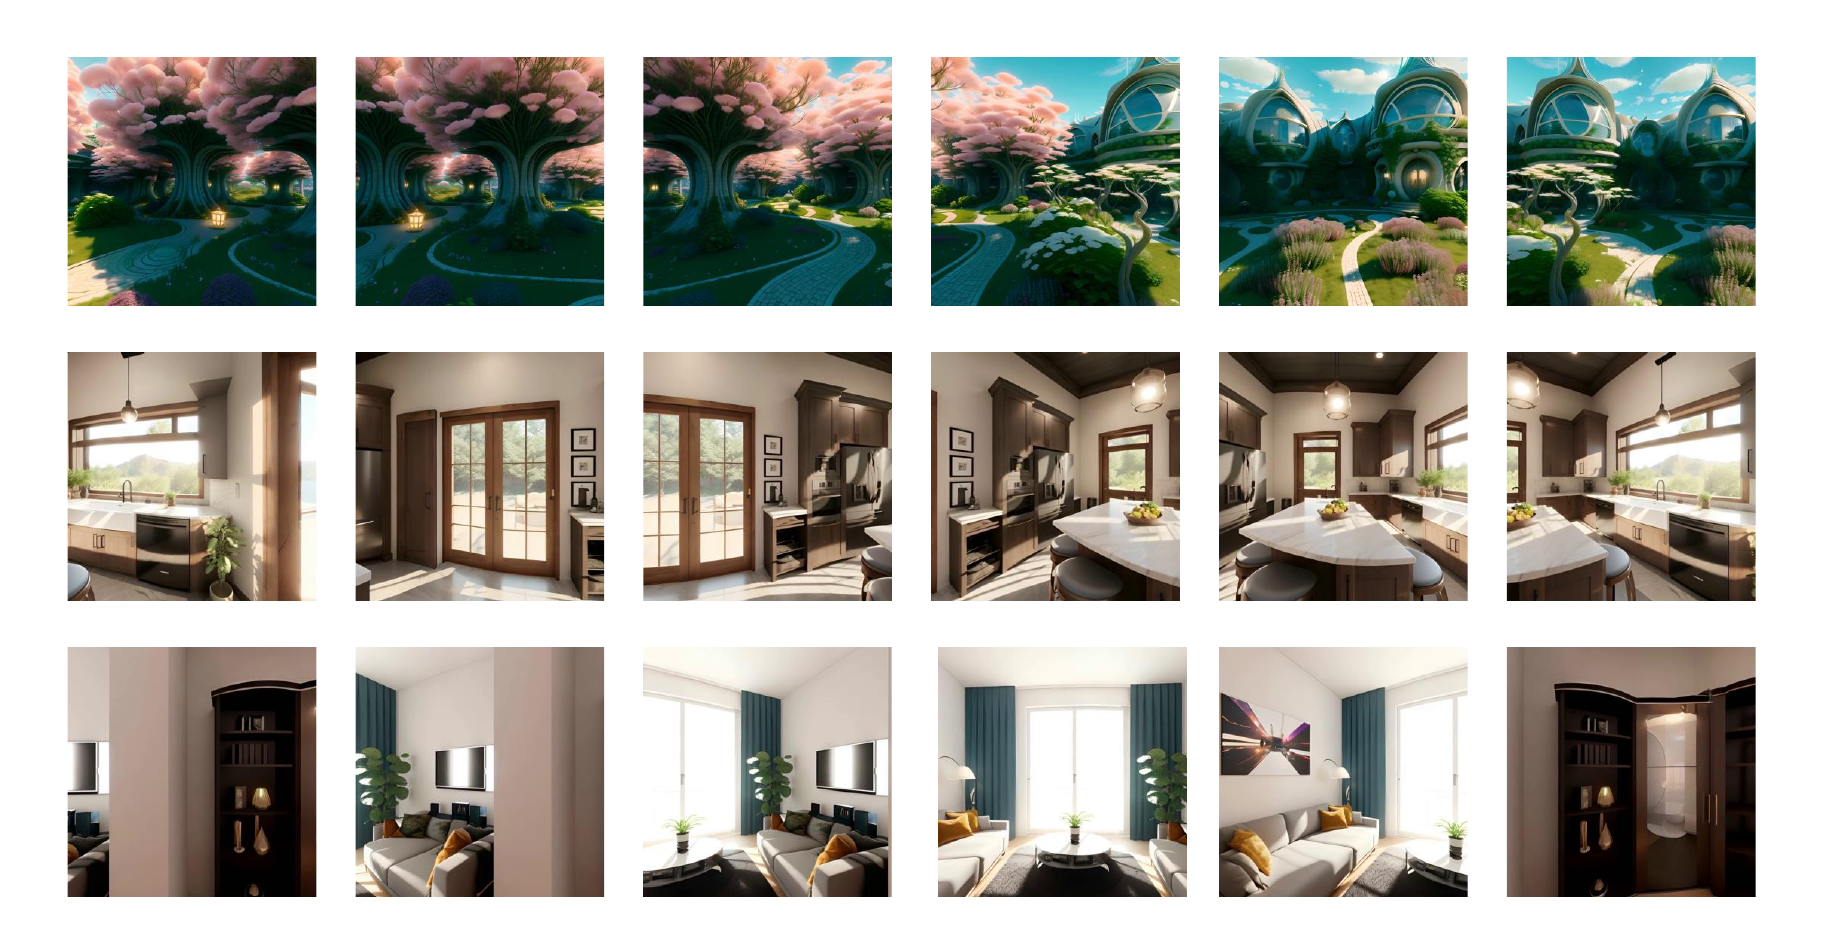}
    \vspace{-3mm}
    \caption{Visualization results of 360-degree scene.}
    \vspace{-2mm}
    \label{fig:3dp_supp}
\end{figure*}
\begin{figure*}[t]
    \centering
    \includegraphics[width=0.9\textwidth]{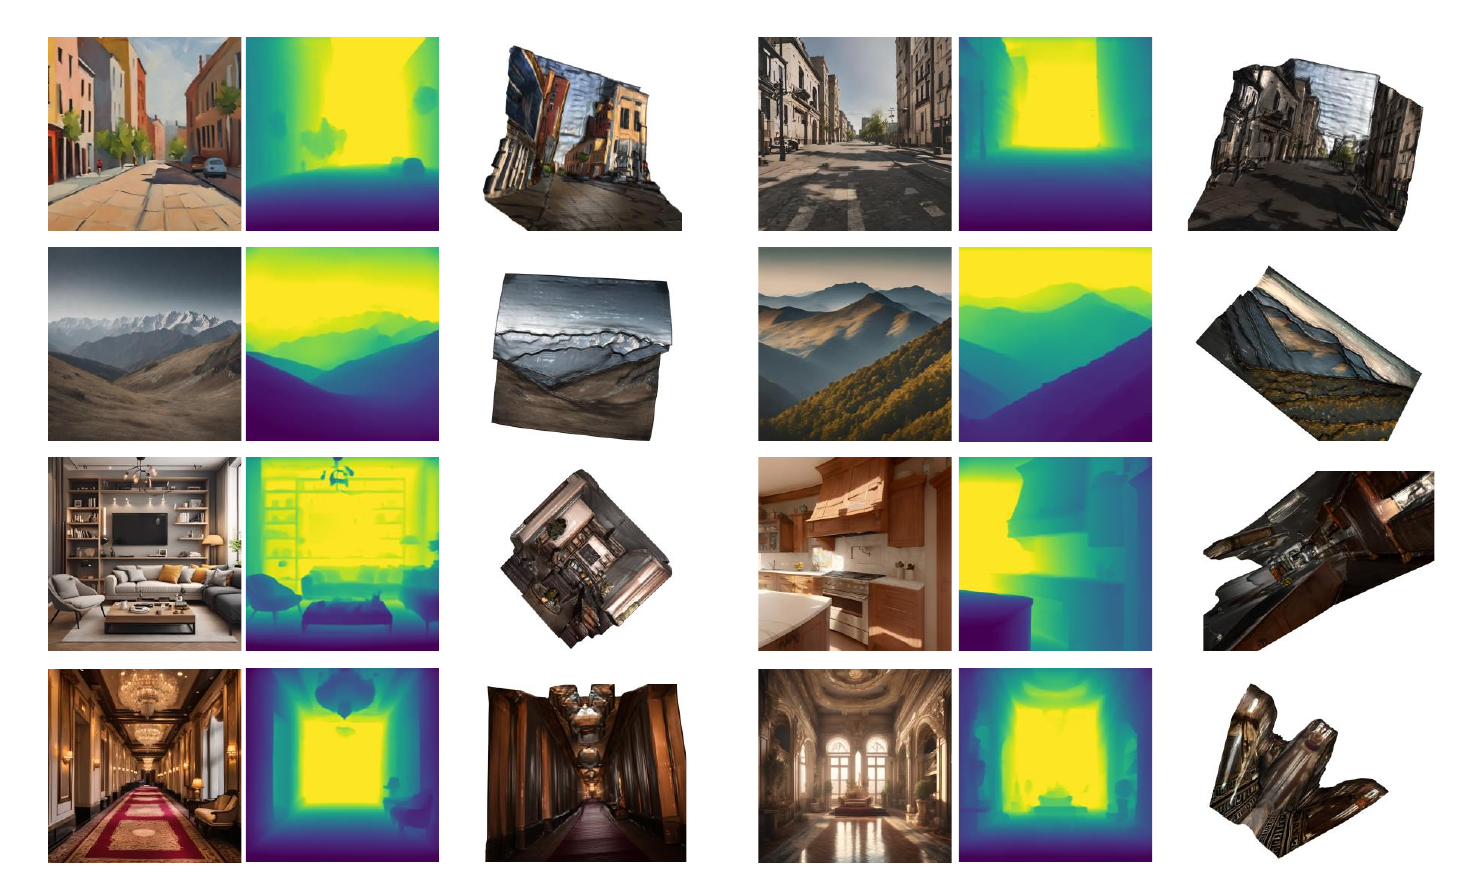}
    \vspace{-3mm}
    \caption{\textbf{Reconstructed 3D Results.} The 3D mesh extracted by marching cube algorithm. Our reconstruction results show that our methods can generate scenes with satisfactory 3D consistency.}
    \vspace{-2mm}
    \label{fig:3d_res}
\end{figure*}
\begin{figure*}[t!]
    \centering
    \includegraphics[width=1.0\textwidth]{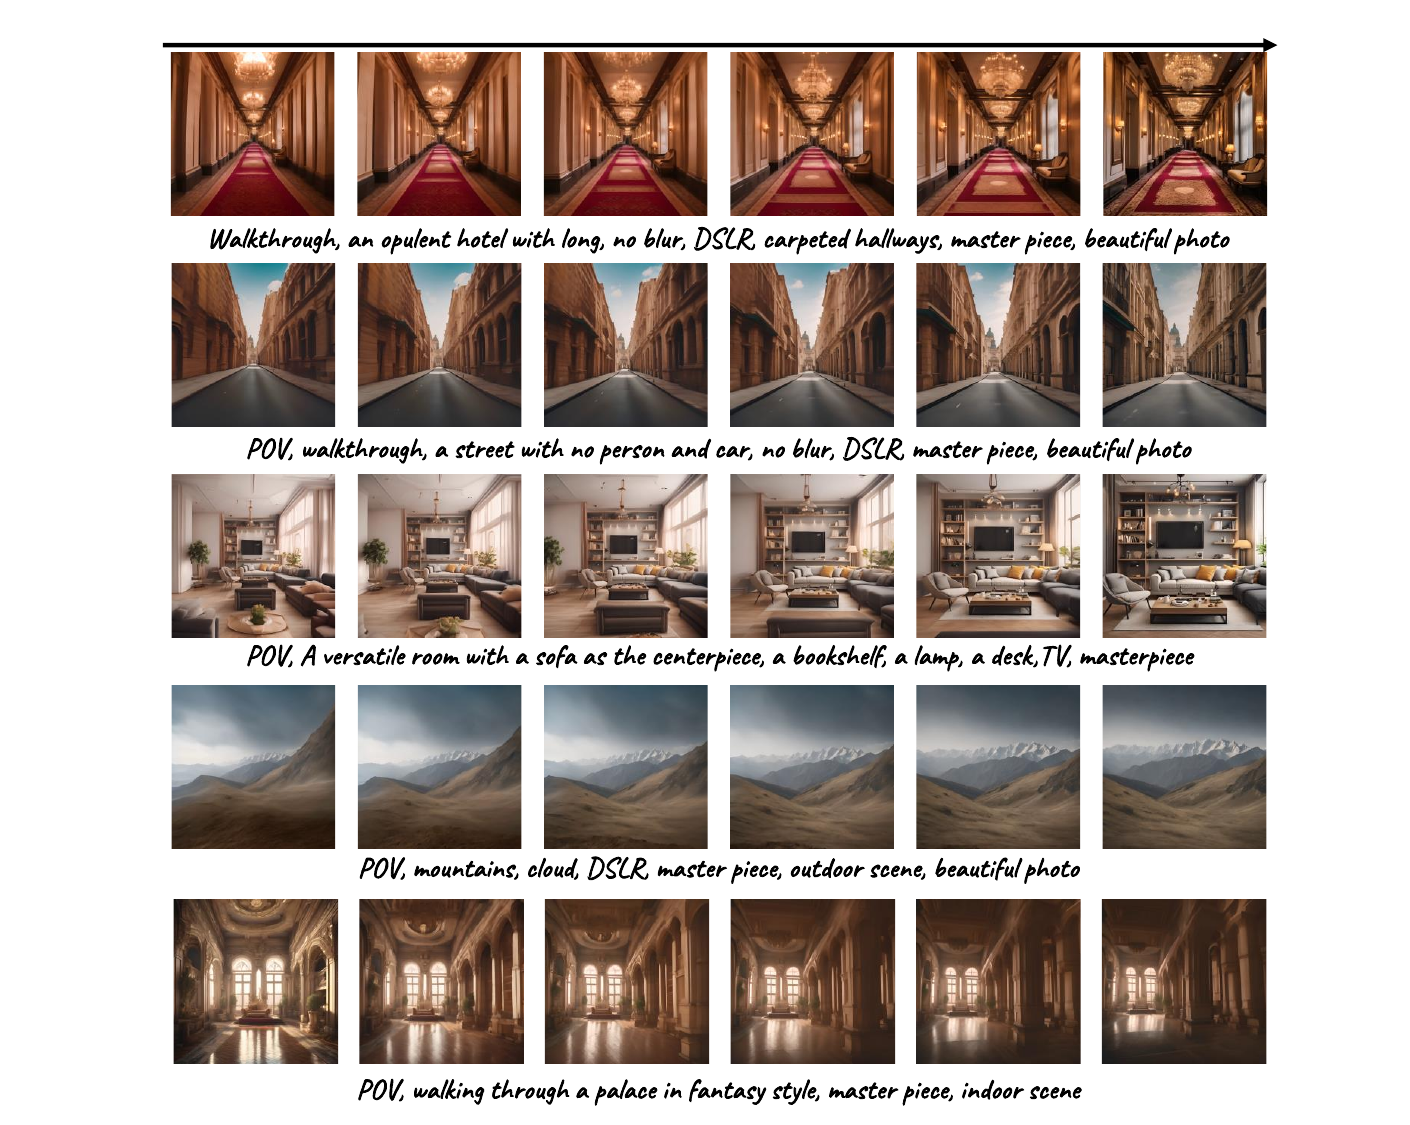}
    % \vspace{-6mm}
    \caption{\textbf{Quantitative Results.} From our results, it can be seen that our approach produces high-fidelity scenes with stable 3D consistency in indoor scenes, outdoor scenes, and unreal-style scenes. More high-resolution results can be found in the supplementary material.}
    % \vspace{-4mm}
    \label{fig:result_supp}
\end{figure*}

\section{Additional Ablation Study Results}
\label{sec:addition_ablation}
\noindent{\textbf{Number of Initial Samples.}}
We explored the impact of the number of samples at scene initialization, on the effectiveness of our method. 
As can be observed in~\cref{tab:ablation_pose_num}, the best results were achieved when the number was at 8. 
We concluded that when the number of initial views is too small, there is a lack of sufficient prior information thus making it difficult to perform high-quality scene initialization. 
However, when there are too many initial samples, the contradiction between the different viewpoints may also lead to a decrease in the quality of the generation because some errors may occur in the image inpainting and depth estimation process.

\noindent{\textbf{Conditional Input of Refine Model.}}
We also explore the design choices of the conditional inputs to the refinement model.
When given the novel view pose, we can get the rendered features, depth, and RGB of the novel viewpoint via volume rendering.
We can then inject the rendered depth, features, or features extracted by the feature adapter into the network, respectively. 
The results in~\cref{tab:ablation_feature} show that the rendered features can be better aligned with the pre-trained feature space of the diffusion model via the feature adapter, giving reasonable guidance for the generation of the new image.

\section{Additional Experimental Results}
\label{sec:addition_exp}

\subsection{Comparsion to Text-to-Object Methods}
We also compare our approach with some Text-to-3D object methods~\cite{dreamfusion, Prolificdreamer, SJC} that can generate NeRF/mesh based on textual prompts. We provide it with a set camera trajectory and some simple textual prompts to generate the 3D scene. Since such methods do not utilize additional depth models to provide geometric information, we compare them only on visual quality metrics.
Given textual prompts and a predefined set of trajectories, these methods~\cite{dreamfusion, Prolificdreamer, SJC} distill the scores of the T2I model to optimize the 3D representation using score distillation sampling~\cite{dreamfusion}.
From the quantitative results in~\cref{fig:text-to-object-supp}, we found that the generated scenes contain a lot of blur and artifacts.
To achieve better visual quality, NeRF typically requires multi-viewpoint observation of the scene from different angles.
Compared to these methods, our approach optimizes NeRF using the generated images with realism, instead of only using score distillation sampling for optimization, and thus achieves more high-fidelity results.
In addition, we also use the depth estimation results to assist the optimization of the 3D representation to learn plausible low-frequency geometrical information, preventing overfitting of high-frequency information in the few-shot setting.

\subsection{Comparision to GEN-1}
To compare to GEN-1, we follow~\cite{scenescape} to use the RealEstate10K dataset, consisting of Internet videos and corresponding camera poses.
We filtered 20 indoor videos that follow a smooth temporal camera motion to adapt it to our setting. 
To do that, we filter videos that adhere to the following constraints:
\begin{equation}
\frac{\left(c_{t+1}-c_t\right)^T v_t}{\left\|\left(c_{t+1}-c_t\right)\right\| \cdot\left\|v_t\right\|} \geq 0.95
\end{equation}
where $c_t$ is the camera center point at frame $t$ and $v_t$ is the viewing direction. 
We subsample the filtered video so that it contains 25 frames.
We can see from~\cref{fig:GEN-1} that even though we have a video clip with 3D consistency as input, the video-to-video translation method still produces inconsistent results.
The main reason for this problem is that such methods lack a unified 3D representation to constrain the output video results.

\subsection{Comparsion to Image-to-3D Methods}
We show some visualization results of the image-guided 3D generation method in~\cref{fig:3dp_supp}.
Specifically, we use T2I models to generate initial images. Subsequently, their pipelines can be used to generate 3D scenes that can be compared to our method. We provide a comprehensive evaluation of these methods based on the 3D consistency and visual quality metrics presented previously.
As can be observed from the visualization results, 3DP does not have the ability to synthesize unseen regions, while many distortions are present in the generated novel view images. 
Whereas Pixelsyn~\cite{pixelsynth} synthesizes many unreasonable views when applied to outdoor scenes due to pre-training on the large-scale indoor dataset only.
These types of methods tend to generate only in-domain data because they are trained with data from a fixed domain, and it is difficult to cope with complex and diverse scenes.

% \section{Additional Discussion on Related Methods}
% \label{sec:addition_discuss}

\section{Limitations}
Our current approach faces challenges primarily due to its computational time and resource requirements. 
The process of scene generation involves continuous optimization of the 3D representation in real-time while simultaneously generating new content through multi-step sampling. 
This iterative process demands substantial computational power and resources.
This is because, during the scene generation process, we need to continually optimize the 3D representation online while generating new content through multi-step sampling.
In the future, this problem may be alleviated by incorporating 3D Gaussian Splatting~\cite{3dgaussian} into our pipeline.

\section{Additional Qualitative Results}
\label{sec:addition_qualitative}
We present some supplementary qualitative results to offer a visual interpretation of the inner workings of our model and to provide insights into its strengths.
We show that our method is capable of handling a wide range of indoor and outdoor scenes as well as Unreal scenes. In addition, our method can also handle arbitrary 6DOF camera trajectories, such as forward, backward, and in-place rotation.
