# Supplementary material for: 3D-SceneDreamer: Text-Driven 3D-Consistent Scene Generation
Source: arXiv:2403.09439 source file (2024-03-14)
Supplement: Supplementary file 2 [file 360_supp.tex]

\begin{figure*}[t]
    \centering
    \includegraphics[width=1.0\textwidth]{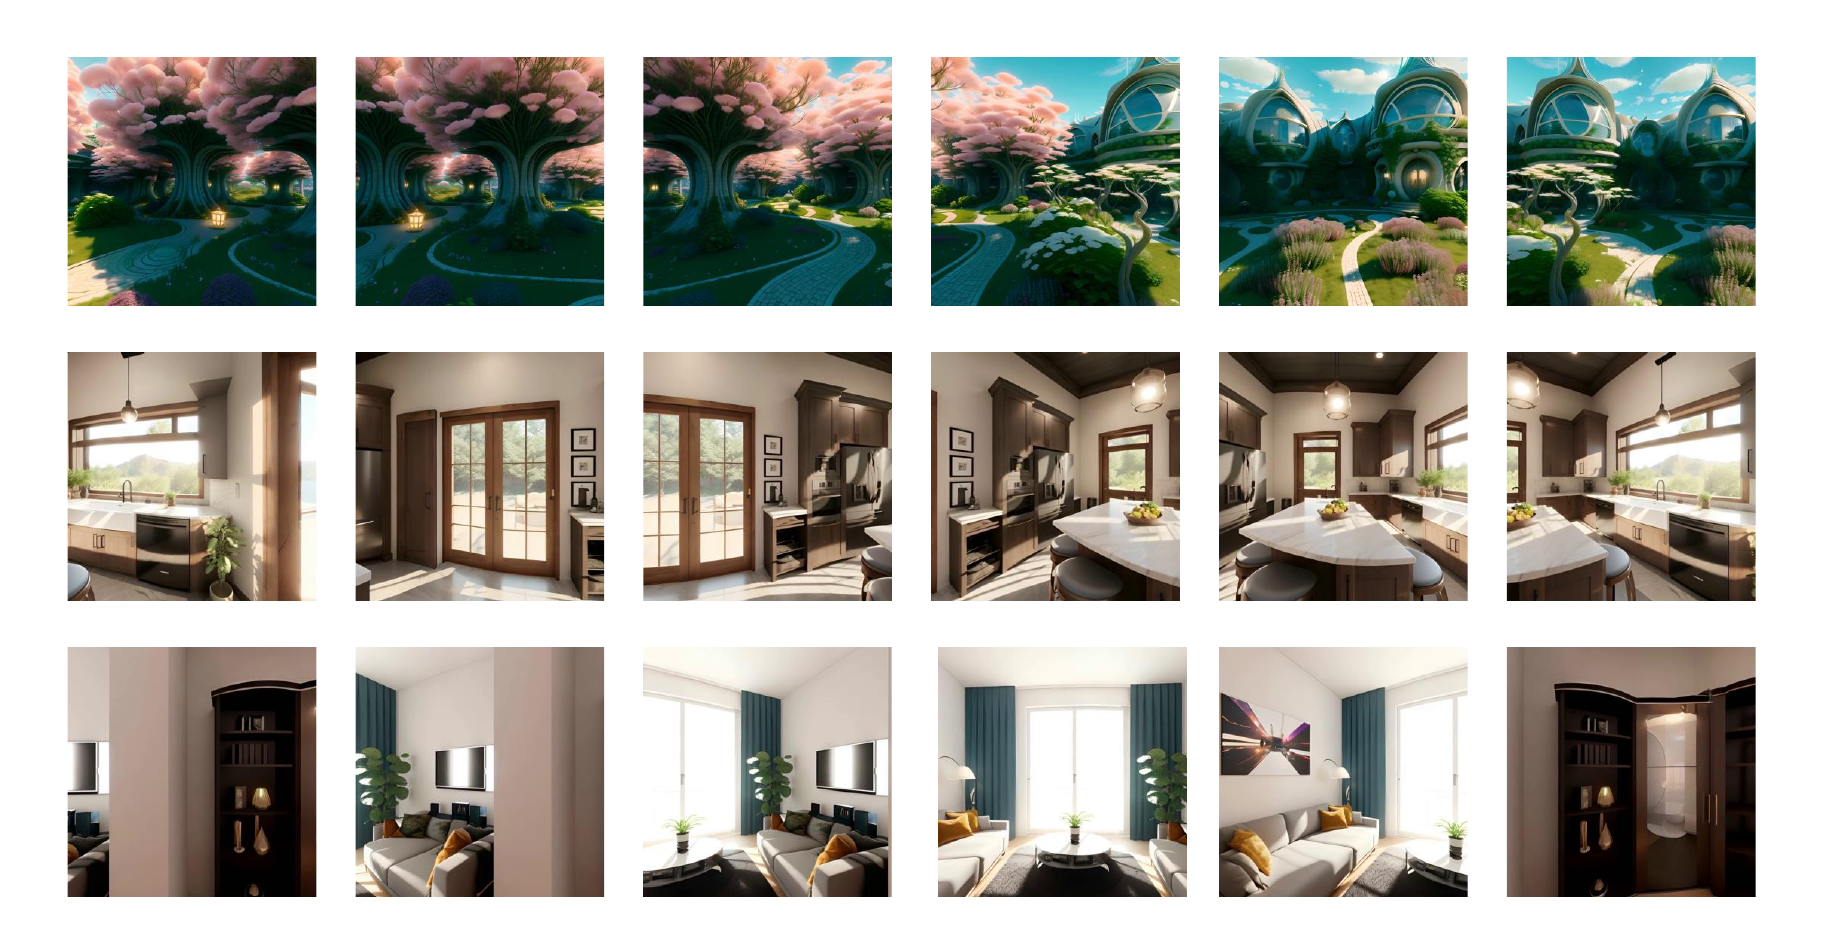}
    \vspace{-3mm}
    \caption{Visualization results of 360-degree scene.}
    \vspace{-2mm}
    \label{fig:3dp_supp}
\end{figure*}
