# Supplementary material for: 3D-SceneDreamer: Text-Driven 3D-Consistent Scene Generation
Source: arXiv:2403.09439 source file (2024-03-14)
Supplement: Supplementary file 4 [file 3dp_result_supp.tex]

\begin{figure}[t]
    \centering
    \includegraphics[width=0.48\textwidth]{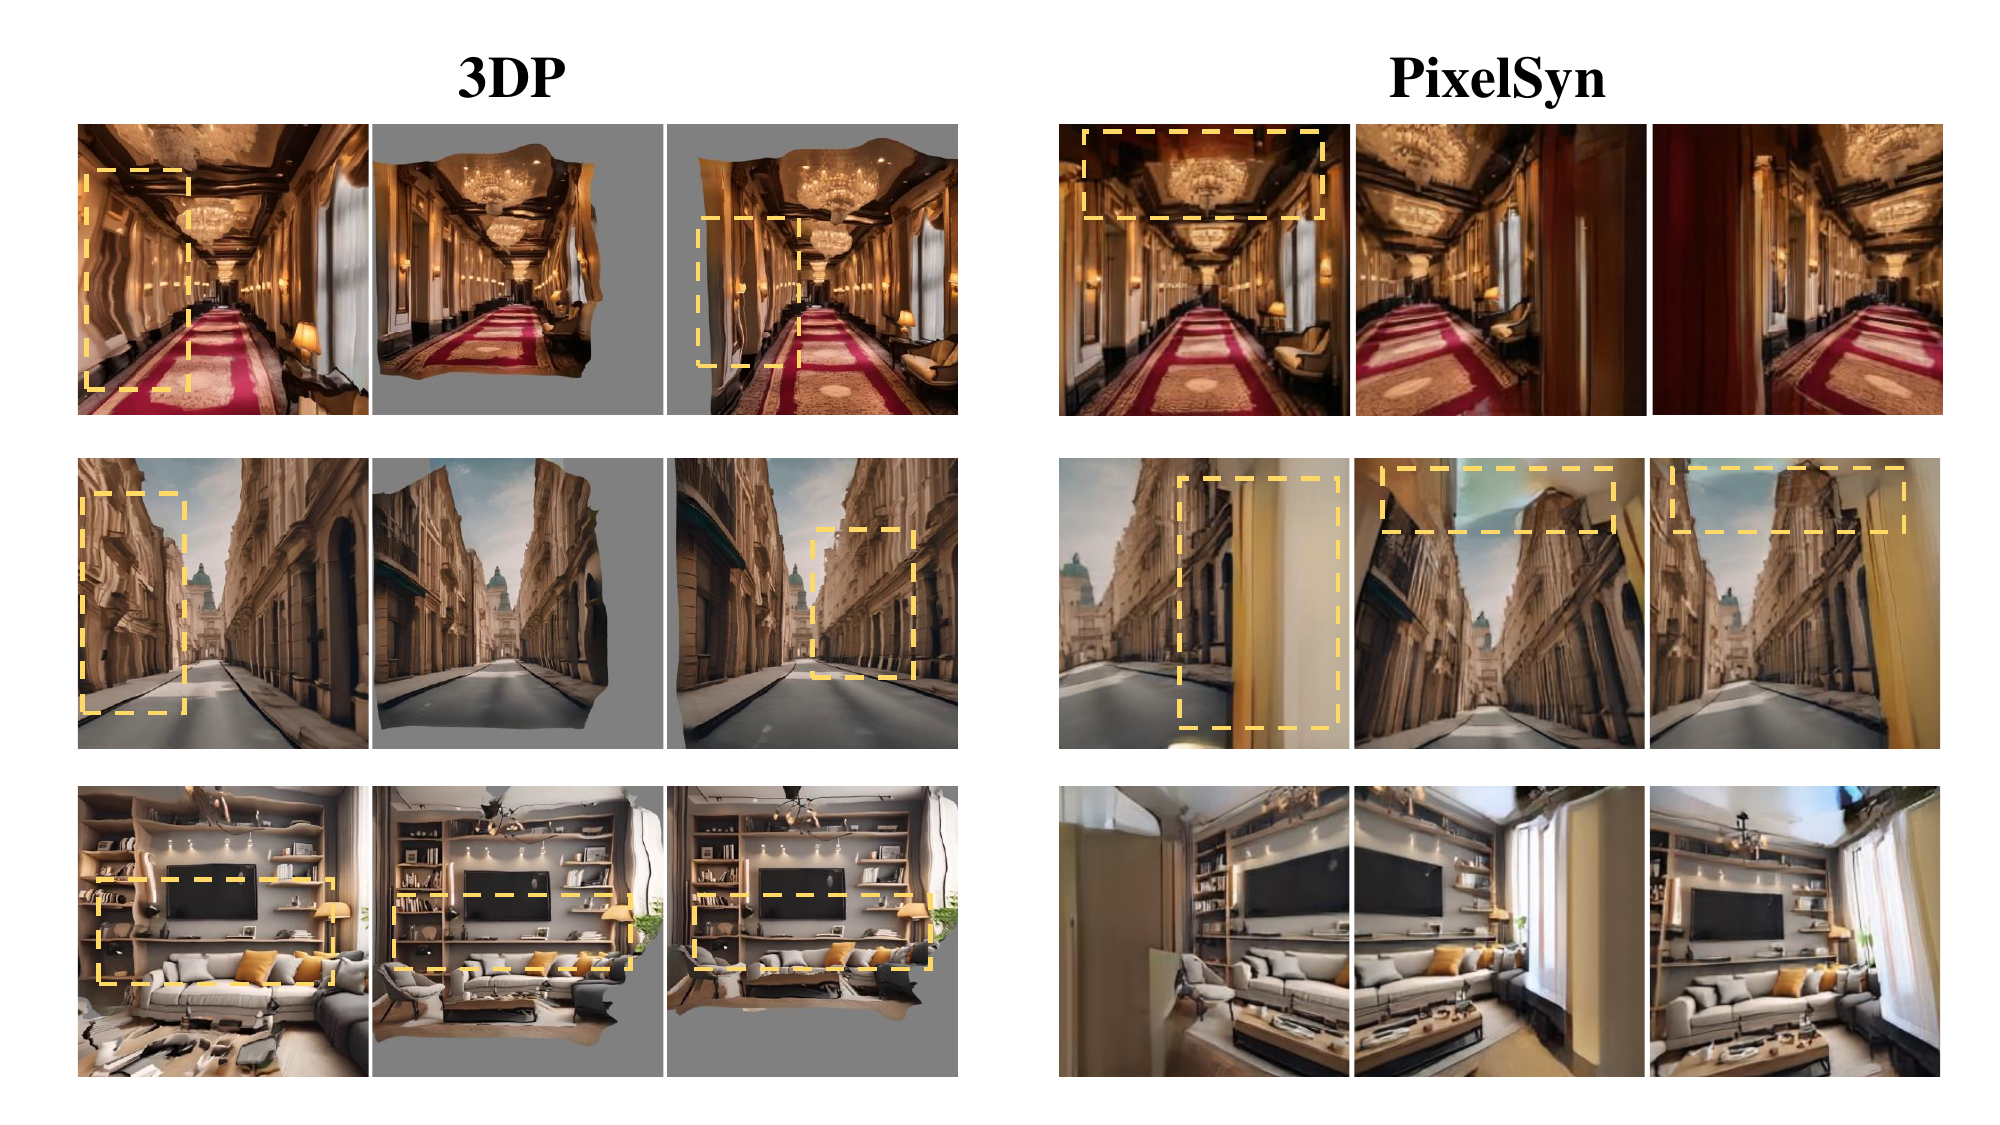}
    \vspace{-3mm}
    \caption{Visualization results of the image-guided scene generation approaches.}
    \vspace{-2mm}
    \label{fig:3dp_supp}
\end{figure}
