# Supplementary material for: 3D-SceneDreamer: Text-Driven 3D-Consistent Scene Generation
Source: arXiv:2403.09439 source file (2024-03-14)
Supplement: Supplementary file 6 [file video_compare_supp.tex]

\begin{figure}[t]
    \centering
    \includegraphics[width=0.48\textwidth]{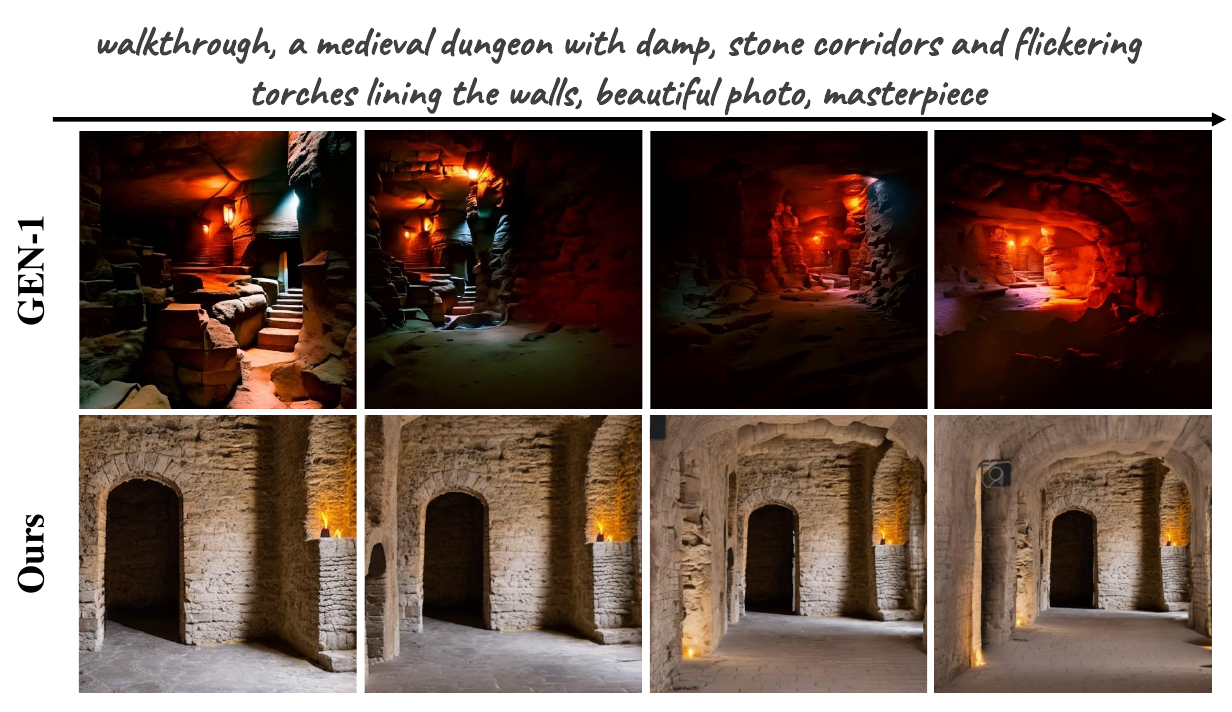}
    \vspace{-2mm}
    \caption{Comparision with video-to-video transition method GEN-1.}
    \vspace{-2mm}
    \label{fig:GEN-1}
\end{figure}
